# Supplementary material for: Experimental quantum teleportation of propagating microwaves
Source: arXiv:2103.04155 ancillary file (2021-03-06)
Supplement: Supplementary file 1 [file Supplementary_Material.pdf]

# Supplementary Material:

# Quantum teleportation of propagating microwaves

K. G. Fedorov,[1,2,*] M. Renger,[1,2] S. Pogorzalek,[1,2,†] R. Di Candia,[3] Q. Chen,[1,2] Y. Nojiri,[1,2] K. Inomata,[4] Y. Nakamura,[4,5] M. Partanen,[1] A. Marx,[1] R. Gross,[1,2,6] and F. Deppe[1,2,6,‡]

[1] *Walther-Meißner-Institut, Bayerische Akademie der Wissenschaften, 85748 Garching, Germany*
[2] *Physik-Department, Technische Universität München, 85748 Garching, Germany*
[3] *Department of Communications and Networking, Aalto University, Espoo, 02150 Finland*
[4] *RIKEN Center for Emergent Matter Science (CEMS), Wako, Saitama 351-0198, Japan*
[5] *Research Center for Advanced Science and Technology (RCAST), The University of Tokyo, Meguro-ku, Tokyo 153-8904, Japan*
[6] *Munich Center for Quantum Science and Technology (MCQST), 80799 Munich, Germany*

(Dated: March 6, 2021)

## SUPPLEMENTARY NOTE 1: EXPERIMENTAL SETUP

The experimental room temperature and cryogenic setup is shown in Supplementary Figure 1. The FPGA and the microwave pump sources for each JPA are pulsed with a data timing generator (DTG). JPA 1 and JPA 2 are both temperature stabilized at 50 mK in order to ensure a stable JPA operation and produce squeezed states with orthogonal squeezing angles. The two squeezed states are superimposed by a cryogenic hybrid ring (50:50 beam splitter) in order to produce path-entangled two-mode squeezed (TMS) states at the outputs of the hybrid ring. By operating JPA 1 and JPA 2 at the same squeezing level, we are able to produce symmetric TMS states with local statistics of a thermal state in each single path. One output path of the beam splitter is connected to a directional coupler while the other one is connected to a cryogenic switch allowing us to either directly detect the signal for characterization purposes or perform quantum teleportation by sending it to another beam splitter. Here, one part of the TMS state is superimposed with the input signal (to-be-teleported signal) and each of the outputs is sent to measurement JPAs (JPA 3 and JPA 4) for strong phase-sensitive amplification with orthogonal amplification angles. Afterwards, another cryogenic switch allows for choosing between a characterization configuration or sending both amplified signals to a third beam splitter. One output of the beam splitter is connected to the coupled port of a directional coupler. For all output lines, the first amplification stage of a high-electron-mobility transistor (HEMT) operating at low temperatures is followed by a room temperature rf-amplifier, which is temperature-stabilized by a Peltier cooler. We use a vector network analyzer for a spectroscopic characterization of the JPAs and a heterodyne detection setup for the tomographic measurements.

The heterodyne detection setup and data processing are similar to those described in Refs. 1 and 2. Here, the signal is roughy filtered around the working frequency and down-converted to 11 MHz by image rejection mixers. The signal is then digitized by a National Instruments NI-5782 transceiver module and processed with a National Instruments PXIe-7975R FPGA module in real time. The digital data processing consists of digital down-conversion (DDC), finite-impulse response (FIR) filtering with a full bandwidth of 400 kHz, and calculation as well as averaging of all quadrature moments $\langle I_1^n I_2^m Q_1^k Q_2^l \rangle$ with $n+m+k+l \leq 4$ for $n, m, k, l \in \mathbb{N}$. During each measurement cycle, the moments of JPAs 1-4 are used to calculate the squeezing angles $\gamma_i^{\mathrm{exp}}$ for each JPA "on the fly" in order to obtain the angle correction $\delta\gamma_i = \gamma_i^{\mathrm{ext}} - \gamma_i^{\mathrm{target}}$ which is used to adjust the phase of the microwave pump tone by $2\delta\gamma_i$. Similarly, the phase of the microwave signal tone is adjusted by $\delta\theta = \theta^{\mathrm{ext}} - \theta^{\mathrm{target}}$ where $\theta$ is the displacement angle of the input coherent state for quantum teleportation. During data analysis on the PC, the recorded traces are separated into different parts according to the DTG timings as indicated in Supplementary Figure 1. The data within a single averaging cycle consists of $7.7 \times 10^8$ raw data points per part of the trace and is used to perform a reference state reconstruction for each pulse in order to obtain the signal moments $\langle (\hat{a}^\dagger)^n \hat{a}^m \rangle$ with $n+m \leq 4$. Finally, this averaging cycle is repeated 10 times. The vector network analyzer, DTG, FPGA card and local oscillator are synchronized to a 10 MHz rubidium frequency standard. The pump microwave sources are daisy chained to the local oscillator with a 1 GHz reference signal.

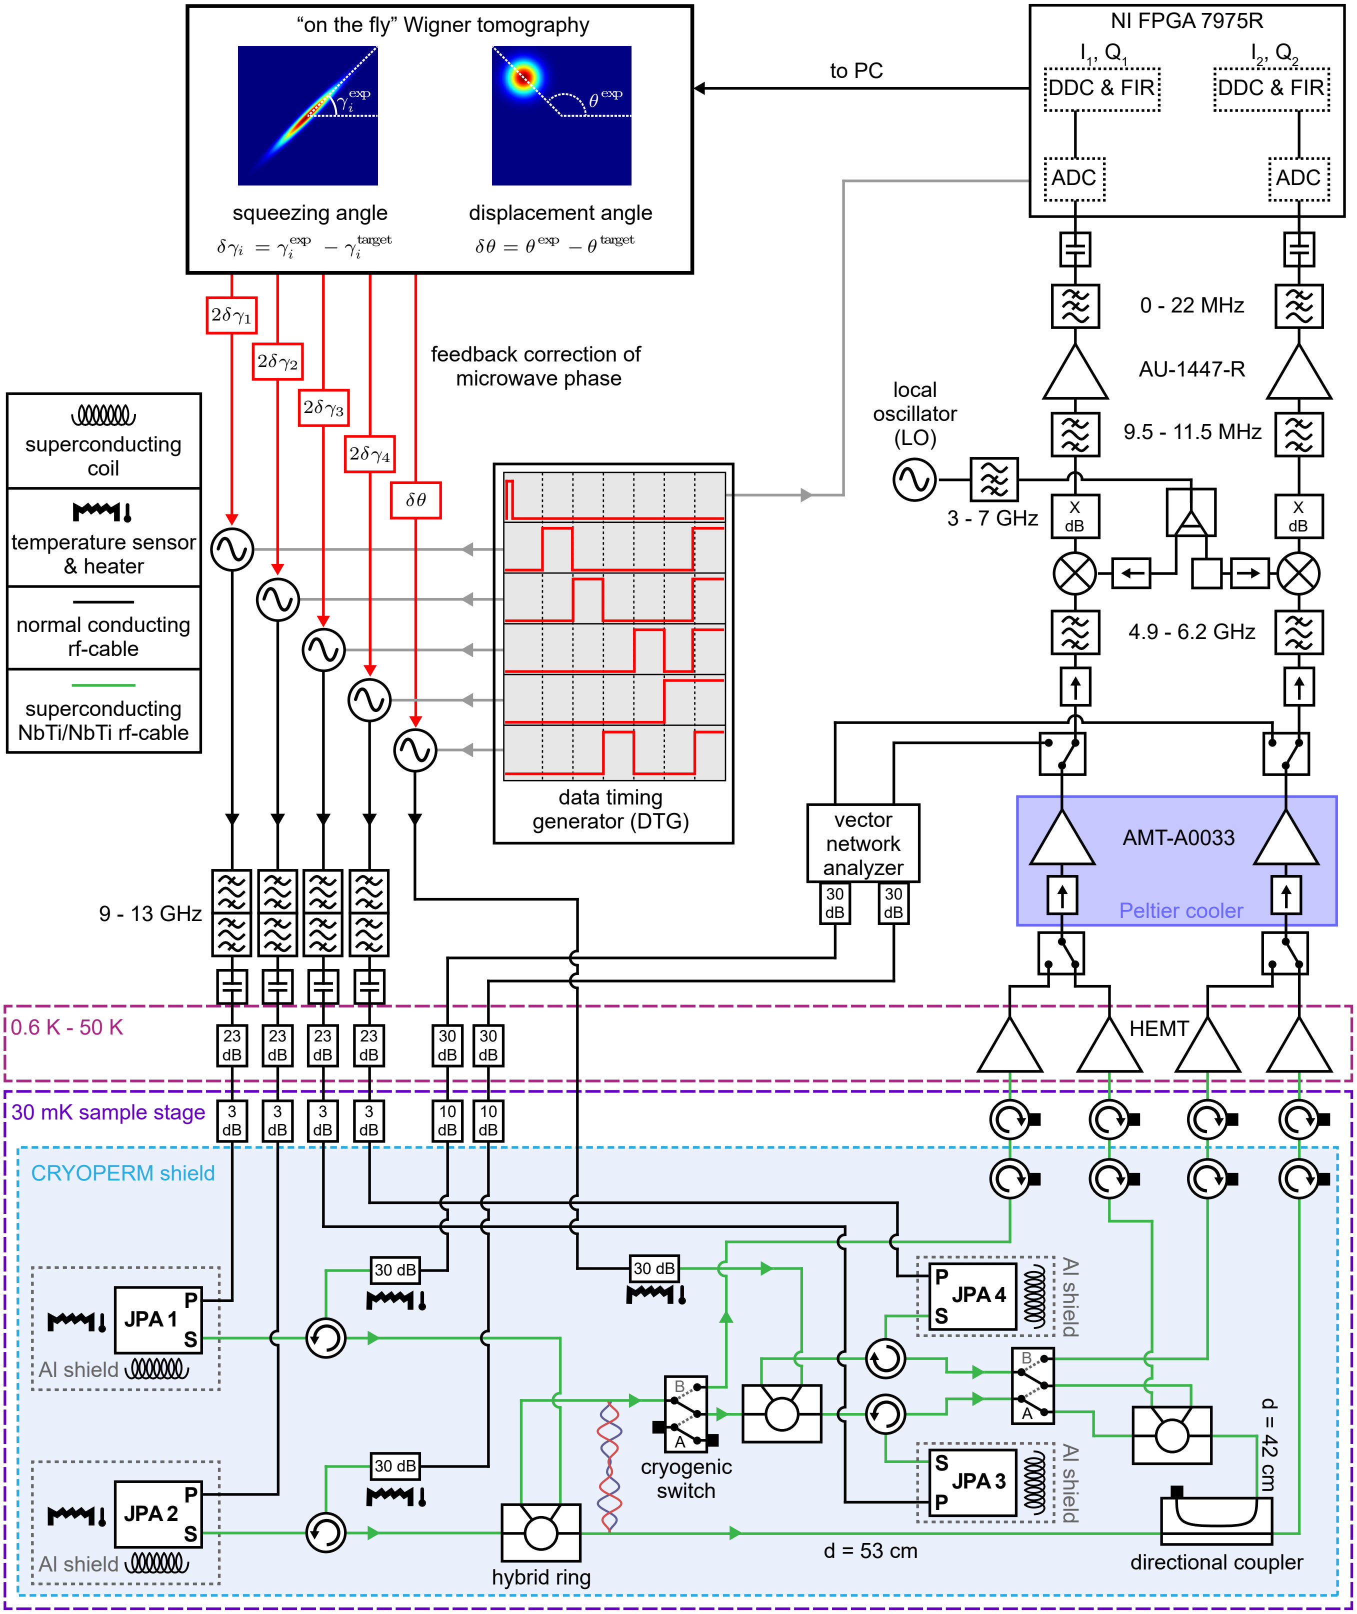


Supplemental Figure 1. Experimental scheme of microwave quantum teleportation protocol with propagating states. The two cryogenic switches allow for quantum teleportation (switch position A) or characterization measurements (switch position B). The intertwined lines between the outputs of the hybrid ring symbolize the entanglement.

# SUPPLEMENTARY NOTE 2: THEORY MODEL

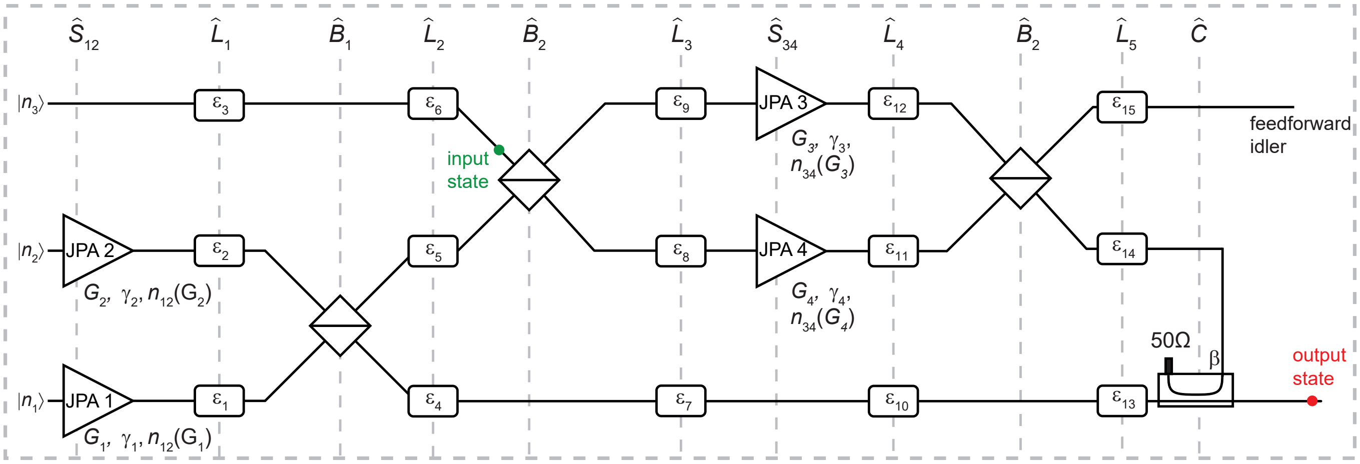


Supplemental Figure 2. Scheme for the iterative simulation of the quantum teleportation protocol. Each iteration step consists either of a unitary operation such as squeezing ($\hat{S}_{12}$, $\hat{S}_{34}$) and beam splitter operations ($\hat{B}_1$, $\hat{B}_2$, $\hat{C}$), or of a non-unitary operation such as path losses ($\hat{L}_1, \hat{L}_2, \hat{L}_3, \hat{L}_4, \hat{L}_5$) and added noise. The squeezing parameter of JPA 1 (JPA 2) is denoted by $r_1$ ($r_2$) and $\gamma_1$ ($\gamma_2$) is the squeezing angle in radians. The degenerate gain of JPA 3 (JPA 4) is described by $G_3$ ($G_4$) and $\gamma_3$ ($\gamma_4$) is the respective squeezing angle in radians. The input state is reconstructed at the position indicated by green dot. Red dot denotes the reconstruction point for the teleported output state.

The quantum teleportation protocol is theoretically modelled in an iterative way, as illustrated in Supplementary Figure 2. The scheme consists of 3 signal paths where path 1 and path 2 form the input for the TMS generation and the input signal is applied at path 3. The weak thermal environment in each path is modelled by the bosonic operator $\hat{f}$ with the average noise photon number

$$\langle \hat{f}^\dagger \hat{f} \rangle = n_{\mathrm{th}} = \frac{1}{e^{\frac{\hbar\omega}{k_{\mathrm{B}}T}} - 1}. \tag{S1}$$

Weak thermal states form inputs for squeezed state generation with JPA 1 and JPA 2 and subsequent path-entanglement at the outputs of the hybrid ring. As a result, the input noise photon numbers $n_1$ and $n_2$ consist of the environmental thermal noise and the noise added by the JPAs, which monotonically increases with increasing degenerate gain $G_i$, $i \in \{1, 2\}$. Based on the existing experimental evidence and related phenomenological theory[3], we assume that this gain dependence obeys a power law

$$n_1 = n_{\mathrm{th}} + \chi_1 (G_1 - 1)^{\chi_2}, \qquad n_2 = n_{\mathrm{th}} + \chi_1 (G_2 - 1)^{\chi_2}. \tag{S2}$$

The initial thermal coherent state $\hat{a}$ with displacement $\alpha$ in path 3 is modelled by applying the displacement operator $\hat{D}(\alpha)$ to the operator $\hat{f}_3$ which describes the initial bosonic noise

$$\hat{a} = \hat{D}(\alpha)^\dagger \hat{f}_3 \hat{D}(\alpha) = \hat{f}_3 + \alpha. \tag{S3}$$

The number of noise photons $n_3$ in the coherent input is quantified by the purity $\mu = 1/(1 + 2n_3)$. As a result, we formally write the input state as $|n_1; n_2; \alpha, \mu\rangle \equiv |n_1\rangle \otimes |n_2\rangle \otimes |\alpha, \mu\rangle$. In each iteration step, we apply either a unitary squeezing/beam splitter operation or a non-unitary operation to model losses and noise. In the first step, a thermal squeezed state is created by JPA 1 and JPA 2. This operation is modelled with the squeezing operator $\hat{S}_{12}$, acting on path 1 and path 2

$$\hat{S}_{12}^\dagger \begin{pmatrix} \hat{a}_1 \\ \hat{a}_2 \\ \hat{a}_3 \end{pmatrix} \hat{S}_{12} = \begin{pmatrix} \hat{a}_1 \cosh r_1 - \hat{a}_1^\dagger e^{-2i\gamma_1} \sinh r_1 \\ \hat{a}_2 \cosh r_2 - \hat{a}_2^\dagger e^{-2i\gamma_2} \sinh r_2 \\ \hat{a}_3 \end{pmatrix}, \tag{S4}$$

where $\hat{a}_j$ is the signal operator in path $j$. In the next step, path 1 and path 2 are entangled with a hybrid ring, which we model as a 50:50 beam splitter by

$$\hat{B}_1^\dagger \begin{pmatrix} \hat{a}_1 \\ \hat{a}_2 \\ \hat{a}_3 \end{pmatrix} \hat{B}_1 = \frac{1}{\sqrt{2}} \begin{pmatrix} \hat{a}_1 + \hat{a}_2 \\ -\hat{a}_1 + \hat{a}_2 \\ \sqrt{2}\,\hat{a}_3 \end{pmatrix}. \tag{S5}$$

The losses are modelled with a beam splitter model according to

$$\hat{L}_j^\dagger \begin{pmatrix} \hat{a}_1 \\ \hat{a}_2 \\ \hat{a}_3 \end{pmatrix} \hat{L}_j = \begin{pmatrix} \sqrt{1-\varepsilon_{3(j-1)+1}}\,\hat{a}_1 + \sqrt{\varepsilon_{3(j-1)+1}}\,\hat{v}_{3(j-1)+1} \\ \sqrt{1-\varepsilon_{3(j-1)+2}}\,\hat{a}_2 + \sqrt{\varepsilon_{3(j-1)+2}}\,\hat{v}_{3(j-1)+2} \\ \sqrt{1-\varepsilon_{3(j-1)+3}}\,\hat{a}_3 + \sqrt{\varepsilon_{3(j-1)+3}}\,\hat{v}_{3(j-1)+3} \end{pmatrix} \tag{S6}$$

with $j \in \{1,2,3,4,5\}$, cf. Supplementary Figure 2. The bosonic bath modes $\hat{v}_{3(j-1)+1}$ model the thermal environment. The power losses are denoted by $\varepsilon_{3(j-1)+3}$ and $\varepsilon_{16}$. The 50:50 beam splitter which entangles path 2 and path 3 is modelled as

$$\hat{B}_2^\dagger \begin{pmatrix} \hat{a}_1 \\ \hat{a}_2 \\ \hat{a}_3 \end{pmatrix} \hat{B}_2 = \frac{1}{\sqrt{2}} \begin{pmatrix} \sqrt{2}\,\hat{a}_1 \\ \hat{a}_2 + \hat{a}_3 \\ -\hat{a}_2 + \hat{a}_3 \end{pmatrix}. \tag{S7}$$

In the next step, JPAs 3 (JPA 4) acts as a degenerate parametric amplifier to realize the Bell measurement by amplifying orthogonal signal quadratures with respective degenerate gain $G_3$ ($G_4$). This amplification process is modelled with a squeezing operator, acting on path 2 and path 3, according to

$$\hat{S}_{34}^\dagger \begin{pmatrix} \hat{a}_1 \\ \hat{a}_2 \\ \hat{a}_3 \end{pmatrix} \hat{S}_{34} = \begin{pmatrix} \hat{a}_1 \\ (\hat{a}_2 + \zeta_3)\cosh r_3 - (\hat{a}_2^\dagger + \zeta_3^*)e^{-2i\gamma_3}\sinh r_3 \\ (\hat{a}_3 + \zeta_4)\cosh r_4 - (\hat{a}_3^\dagger + \zeta_4^*)e^{-2i\gamma_4}\sinh r_4 \end{pmatrix}, \tag{S8}$$

where the squeezing parameters $r_3$ ($r_4$) are related to the degenerate gain via $G_3 = e^{2r_3}$ ($G_4 = e^{2r_4}$) and the squeezing angle of JPA 3 (JPA 4) is denoted by $\gamma_3$ ($\gamma_4$). In the following, we assume equal degenerate gain for both JPAs, $G_3 = G_4 = G$. The noise added by JPA 3 (JPA 4) is modelled with a random classical variable $\zeta_3$ ($\zeta_4$). We assume that JPA 3 and JPA 4 have equal noise properties, $\zeta_3 = \zeta_4 = \zeta$ and assume $\zeta$ to obey a centralized Gaussian distribution with $\langle \zeta\zeta^* \rangle = n_{34}(G)$ and $\langle \mathrm{Re}(\zeta^2) \rangle = \langle \mathrm{Im}(\zeta^2) \rangle = n_{34}(G)/2$. Similar as in Supplementary Eq. S2, we assume that the JPA noise depends on the gain $G$ as

$$n_{34}(G) = \chi_1 (G-1)^{\chi_2}, \tag{S9}$$

where $\chi_1$ and $\chi_2$ are phenomenological constants characterizing noise properties of the JPAs. The displacement operation for Bob's quantum state in path 1 is realized by a directional coupler, acting as an asymmetric beam splitter with a reflectivity $\beta$

$$\hat{C}^\dagger \begin{pmatrix} \hat{a}_1 \\ \hat{a}_2 \\ \hat{a}_3 \end{pmatrix} \hat{C} = \begin{pmatrix} \sqrt{1-\beta}\,\hat{a}_1 + \sqrt{\beta}\,\hat{a}_2 \\ -\sqrt{\beta}\,\hat{a}_1 + \sqrt{1-\beta}\,\hat{a}_2 \\ \hat{a}_3 \end{pmatrix}. \tag{S10}$$

In the ideal case, as it will be shown later, $\beta$ needs to fulfill the analog teleportation condition $\beta = 4/[g(1-\varepsilon)]$, where $\varepsilon$ models the path losses after JPA 3 and JPA 4. Finally, the teleportation protocol can be expressed by the operator

$$\hat{T} = \hat{C}\hat{L}_5\hat{B}_2\hat{L}_4\hat{S}_{34}\hat{L}_3\hat{B}_2\hat{L}_2\hat{B}_1\hat{L}_1\hat{S}_{12}, \tag{S11}$$

and the final state $|\Psi\rangle$ is given by

$$|\Psi\rangle = \hat{T}|n_1; n_2; \alpha, n_3\rangle. \tag{S12}$$

The moments of the output signal $\hat{b}$ can then be calculated by

$$\begin{pmatrix} \langle(\hat{b}^\dagger)^n \hat{b}^m\rangle_1 \\ \langle(\hat{b}^\dagger)^n \hat{b}^m\rangle_2 \\ \langle(\hat{b}^\dagger)^n \hat{b}^m\rangle_3 \end{pmatrix} = \langle\Psi| \begin{pmatrix} \langle(\hat{a}^\dagger)^n \hat{a}^m\rangle_1 \\ \langle(\hat{a}^\dagger)^n \hat{a}^m\rangle_2 \\ \langle(\hat{a}^\dagger)^n \hat{a}^m\rangle_3 \end{pmatrix} |\Psi\rangle. \tag{S13}$$

We assume that all quantum states are Gaussian, which implies that only moments up to second order are required for full state tomography. As a result, it is sufficient to analyze the effect of the teleportation protocol on the respective displacement vector $d$ and covariance matrix $V$. We realize this by rewriting Supplementary Eq.S13 specifically for the first- and second-order quadrature moments. For the initial displacement vector $d_0$, we have

$$d_0 = (0,\ 0,\ 0,\ 0,\ \sqrt{n_\mathrm{d}}\cos\varphi_\mathrm{d},\ \sqrt{n_\mathrm{d}}\sin\varphi_\mathrm{d})^\mathrm{T} \tag{S14}$$

where $n_\mathrm{d}$ is the number of displacement photons and $\varphi_\mathrm{d}$ describes the displacement angle. In the following, $I_2$ denotes the $2\times 2$ identity matrix and $0_2$ is the $2\times 2$ zero matrix. For the initial covariance matrix, we write

$$V_0 = \frac{1}{4}\begin{pmatrix}(1+2n_1)I_2 & 0_2 & 0_2\\ 0_2 & (1+2n_2)I_2 & 0_2\\ 0_2 & 0_2 & (1+2n_3)I_2\end{pmatrix}. \tag{S15}$$

The squeeze operation for JPA 1 and JPA 2 is modelled by

$$S_{12} = \underbrace{\begin{pmatrix} e^{-r_1} & 0 & 0 & 0 & 0 & 0\\ 0 & e^{r_1} & 0 & 0 & 0 & 0\\ 0 & 0 & e^{-r_2} & 0 & 0 & 0\\ 0 & 0 & 0 & e^{r_2} & 0 & 0\\ 0 & 0 & 0 & 0 & 1 & 0\\ 0 & 0 & 0 & 0 & 0 & 1\end{pmatrix}}_{\text{Squeezing with } r_1, r_2} \cdot \underbrace{\begin{pmatrix} \cos 2\gamma_1 & \sin 2\gamma_1 & 0 & 0 & 0 & 0\\ -\sin 2\gamma_1 & \cos 2\gamma_1 & 0 & 0 & 0 & 0\\ 0 & 0 & \cos 2\gamma_2 & \sin 2\gamma_2 & 0 & 0\\ 0 & 0 & -\sin 2\gamma_2 & \cos 2\gamma_2 & 0 & 0\\ 0 & 0 & 0 & 0 & 1 & 0\\ 0 & 0 & 0 & 0 & 0 & 1\end{pmatrix}}_{\text{Rotation by } 2\gamma_1, 2\gamma_2}. \tag{S16}$$

The beam splitter operations can be expressed as

$$B_2 = \frac{1}{\sqrt{2}}\begin{pmatrix}\sqrt{2}I_2 & 0_2 & 0_2\\ 0_2 & I_2 & I_2\\ 0_2 & -I_2 & I_2\end{pmatrix}, \qquad B_1 = \frac{1}{\sqrt{2}}\begin{pmatrix} I_2 & I_2 & 0_2\\ -I_2 & I_2 & 0_2\\ 0_2 & 0_2 & \sqrt{2}\, I_2\end{pmatrix}. \tag{S17}$$

To model the phase-sensitive amplification of JPA 3 and JPA 4, we define the matrices

$$S_3 = \underbrace{\begin{pmatrix} 1 & 0 & 0 & 0 & 0 & 0\\ 0 & 1 & 0 & 0 & 0 & 0\\ 0 & 0 & 1/\sqrt{G_3} & 0 & 0 & 0\\ 0 & 0 & 0 & \sqrt{G_3} & 0 & 0\\ 0 & 0 & 0 & 0 & 1 & 0\\ 0 & 0 & 0 & 0 & 0 & 1\end{pmatrix}}_{\text{Amplification with degenerate gain } G_3}, \qquad R_3 = \underbrace{\begin{pmatrix} 1 & 0 & 0 & 0 & 0 & 0\\ 0 & 1 & 0 & 0 & 0 & 0\\ 0 & 0 & \cos 2\gamma_3 & \sin 2\gamma_3 & 0 & 0\\ 0 & 0 & -\sin 2\gamma_3 & \cos 2\gamma_3 & 0 & 0\\ 0 & 0 & 0 & 0 & 1 & 0\\ 0 & 0 & 0 & 0 & 0 & 1\end{pmatrix}}_{\text{Rotation by } 2\gamma_3}, \tag{S18}$$

and

$$S_4 = \underbrace{\begin{pmatrix} 1 & 0 & 0 & 0 & 0 & 0\\ 0 & 1 & 0 & 0 & 0 & 0\\ 0 & 0 & 1 & 0 & 0 & 0\\ 0 & 0 & 0 & 1 & 0 & 0\\ 0 & 0 & 0 & 0 & 1/\sqrt{G_4} & 0\\ 0 & 0 & 0 & 0 & 0 & \sqrt{G_4}\end{pmatrix}}_{\text{Amplification with degenerate gain } G_4}, \qquad R_4 = \underbrace{\begin{pmatrix} 1 & 0 & 0 & 0 & 0 & 0\\ 0 & 1 & 0 & 0 & 0 & 0\\ 0 & 0 & 1 & 0 & 0 & 0\\ 0 & 0 & 0 & 1 & 0 & 0\\ 0 & 0 & 0 & 0 & \cos 2\gamma_4 & \sin 2\gamma_4\\ 0 & 0 & 0 & 0 & -\sin 2\gamma_4 & \cos 2\gamma_4\end{pmatrix}}_{\text{Rotation by } 2\gamma_4}. \tag{S19}$$

The phase-sensitive amplification of JPA 3 and JPA 4 is then described by the matrices

$$J_3 = R_3^\dagger S_3 R_3, \qquad J_4 = R_4^\dagger S_4 R_4. \tag{S20}$$

The noise added by JPA 3 and JPA 4 is described by

$$N_3 = \frac{n_{34}(G_3)}{2}\begin{pmatrix}0_2 & 0_2 & 0_2\\ 0_2 & I_2 & 0_2\\ 0_2 & 0_2 & 0_2\end{pmatrix}, \qquad N_4 = \frac{n_{34}(G_4)}{2}\begin{pmatrix}0_2 & 0_2 & 0_2\\ 0_2 & 0_2 & 0_2\\ 0_2 & 0_2 & I_2\end{pmatrix}. \tag{S21}$$

To model the losses, we define the corresponding matrices

$$L_j = \begin{pmatrix} \sqrt{1-\varepsilon_{3(j-1)+1}}\, I_2 & 0_2 & 0_2 \\ 0_2 & \sqrt{1-\varepsilon_{3(j-1)+2}}\, I_2 & 0_2 \\ 0_2 & 0_2 & \sqrt{1-\varepsilon_{3(j-1)+3}}\, I_2 \end{pmatrix} \tag{S22}$$

and

$$A_j = \frac{1}{4}(1+2n_{\mathrm{th}}) \begin{pmatrix} \varepsilon_{3(j-1)+1} I_2 & 0_2 & 0_2 \\ 0_2 & \varepsilon_{3(j-1)+2} I_2 & 0_2 \\ 0_2 & 0_2 & \varepsilon_{3(j-1)+3} I_2 \end{pmatrix}. \tag{S23}$$

with $j \in \{1,2,3,4,5\}$. For the directional coupler, we write

$$C = \begin{pmatrix} \sqrt{1-\beta}\, I_2 & \sqrt{\beta}\, I_2 & 0_2 \\ -\sqrt{\beta}\, I_2 & \sqrt{1-\beta}\, I_2 & 0_2 \\ 0_2 & 0_2 & I_2 \end{pmatrix}. \tag{S24}$$

We define

$$T = CL_5 B_2 L_4 J_3 J_4 L_3 B_2 L_2 B_1 L_1 S_{12}. \tag{S25}$$

The displacement $d'$ after the directional coupler can then be calculated by

$$d' = T d_0. \tag{S26}$$

For the covariance matrix $V'$ of the final state, we find the expression

$$V' = TV_0 T^\dagger + A, \tag{S27}$$

where the added matrix $A$ can be analytically expressed as

$$A = CL_5 B_2 L_4 J_4 J_3 L_3 B_2 L_2 B_1 A_1 B_1^\dagger L_2^\dagger B_2^\dagger L_3^\dagger J_3^\dagger J_4^\dagger L_4^\dagger B_2^\dagger L_5^\dagger C^\dagger \tag{S28}$$
$$+ CL_5 B_2 L_4 J_4 J_3 L_3 B_2 A_2 B_2^\dagger L_3^\dagger J_3^\dagger J_4^\dagger L_4^\dagger B_2^\dagger L_5^\dagger C^\dagger \tag{S29}$$
$$+ CL_5 B_2 L_4 J_4 J_3 A_3 J_3^\dagger J_4^\dagger L_4^\dagger B_2^\dagger L_5^\dagger C^\dagger \tag{S30}$$
$$+ CL_5 B_2 L_4 J_4 N_3 J_4^\dagger L_4^\dagger B_2^\dagger L_5^\dagger C^\dagger \tag{S31}$$
$$+ CL_5 B_2 L_4 N_4 L_4^\dagger B_2^\dagger L_5^\dagger C^\dagger \tag{S32}$$
$$+ CL_5 B_2 A_4 B_2^\dagger L_5^\dagger C^\dagger \tag{S33}$$
$$+ CA_5 C^\dagger. \tag{S34}$$

The displacement for the reference input state is calculated by

$$d = L_2 B_1 L_1 S_{12} d_0. \tag{S35}$$

We rewrite $d'$ and $d_{\mathrm{i}}$ as

$$d' = \begin{pmatrix} d_1' \\ d_2' \\ d_3' \end{pmatrix}, \qquad d = \begin{pmatrix} d_1 \\ d_2 \\ d_3 \end{pmatrix}. \tag{S36}$$

The covariance matrix of the input state is given by

$$V = L_2 B_1 L_1 S_{12} V_0 S_{12}^\dagger L_1^\dagger B_1^\dagger L_2^\dagger + A_{\mathrm{i}} \tag{S37}$$

with

$$A_{\mathrm{i}} = L_2 B_1 A_1 B_1^\dagger L_2^\dagger + A_2. \tag{S38}$$

We rewrite the resulting covariance matrices in block form

$$V' = \left(\begin{array}{c|c|c} V_1' & * & * \\ \hline * & V_2' & * \\ \hline * & * & V_3' \end{array}\right) \qquad V = \left(\begin{array}{c|c|c} V_1 & * & * \\ \hline * & V_2 & * \\ \hline * & * & V_3 \end{array}\right), \tag{S39}$$

where $V_j'$ denotes the final covariance matrix in path $j$ and $V_j$ denotes the respective input covariance matrix . In the next step, we calculate the Uhlmann-fidelity between the states $(d_3, V_3)$ and $(d_1', V_1')$, which can be expressed for single mode Gaussian states as

$$F(d_3, V_3, d_1', V_1') = \frac{1}{2}\frac{\exp(-\boldsymbol{\beta}^{\mathrm{T}}(V_3 + V_1')^{-1}\boldsymbol{\beta})}{\sqrt{\Lambda + \Delta} - \sqrt{\Delta}}, \tag{S40}$$

where $\Lambda = \det(V_3 + V_1')$, $\Delta = 16(\det V_3 - 1/16)(\det V_1' - 1/16)$ and $\boldsymbol{\beta} = d_3 - d_1'$. To fit the experimental data, as shown in Fig. 3 in the main text, we use a least-square fit, where the JPA noise coefficients $\chi_1$, $\chi_2$, and the environmental temperature $T$ are treated as fit parameters. As a result, we minimize the squared distance between the experimentally determined fidelities $\{F(r_i, G_i)\}$ for squeezing $r_i$ and degenerate gain $G_i$ and the theoretically predicted values $F_{\mathrm{t}}(\chi_1, \chi_2, T, \{\mathbf{x}_i\})$, where $\chi_1$, $\chi_2$, and $T$ are treated as variables and $\{\mathbf{x}_i\}$ is the parameter set including the JPA 1 and JPA 2 squeezing parameters $r_i$, the degenerate gain $G_i$ of JPA 3 and JPA 4, the amplification angles $\gamma_i$ as well as the constant system parameters such as path losses, and coupling strength $\beta$. Thus, we fit the measurement data by minimizing the function

$$\mathcal{L}(\chi_1, \chi_2, T, \{\mathbf{x}\}, \{F_i\}) = \sum_i |F_{\mathrm{t}}(\chi_1, \chi_2, T, \{\mathbf{x}\}) - F(r_i, G_i)|^2. \tag{S41}$$

The parameters used in the numerical model are summarized in Tab. I. The parameters $\chi_1$, $\chi_2$, and $T$ are extracted from the fit routine and the losses are estimated from the data sheets of the respective passive microwave components. The loss values $\varepsilon_3$, $\varepsilon_6$, $\varepsilon_7$, $\varepsilon_{10}$ and $\varepsilon_{13}$ are set to zero since they have been artificially introduced to keep the block matrix structure which simplifies the numerical calculation.

Supplemental Table I. Model parameters used for the QT protocol fit in the main article. The loss values $\varepsilon_i$ are estimated from individual losses of various components. During the fit we have varied three parameteres, $\chi_1$, $\chi_2$, and $T$.

| $\chi_1$ | $\chi_2$ | $T$ (mK) | $\beta$ (dB) | $\varepsilon_1$ (dB) | $\varepsilon_2$ (dB) | $\varepsilon_3$ (dB) |
|---|---|---|---|---|---|---|
| 0.0397 | 0.2428 | 73.7 | -15 | 0.36 | 0.35 | 0 |
| $\varepsilon_4$ (dB) | $\varepsilon_5$ | $\varepsilon_6$ (dB) | $\varepsilon_7$ (dB) | $\varepsilon_8$ (dB) | $\varepsilon_9$ (dB) | $\varepsilon_{10}$ (dB) |
| 0.5 | 1.1 | 0 | 0 | 0.64 | 0.63 | 0 |
| $\varepsilon_{11}$ (dB) | $\varepsilon_{12}$ (dB) | $\varepsilon_{13}$ (dB) | $\varepsilon_{14}$ (dB) | $\varepsilon_{15}$ (dB) | $f_0$ (GHz) | $n_{\mathrm{d}}$ |
| 0.84 | 0.88 | 0 | 0.5 | 0.7 | 5.435 | 1.1 |
| $\mu$ | | | | | | |
| 0.98 | | | | | | |

## SUPPLEMENTARY NOTE 3: BELL DETECTION

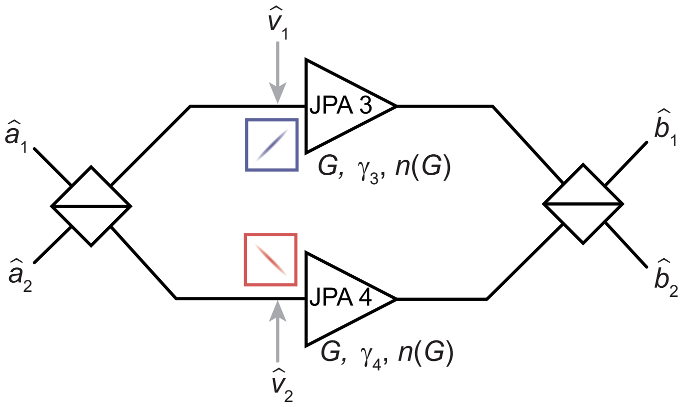


Supplemental Figure 3. Josephson mixer, consisting of JPA 3 and JPA 4 to realize the Bell detection.

Alice measures her two-mode Gaussian state with the Josephson mixer setup shown in Fig. 3. The projective character of this measurement depends sensitively on the choice of the coupling factor $\beta$ of the subsequent directional coupler (shown in Fig. 2) and the degenerate gain $G$ of JPA 3 and JPA 4. In the following, we show that the quantity $G\beta$ allows us to distinguish between coherent state quantum teleportation and vacuum teleportation. In the limit $\beta \to 0$, $G \to \infty$, Alice's state detection becomes ideally projective if $G\beta = 4$. Simultaneously, the regime of vacuum teleportation is characterized by $G \to 1$. For $G\beta \gg 4$, the measurement apparatus acts as an amplifier, leading to imperfect interference at the directional coupler. To investigate these regimes, we consider the ideal quantum teleportation protocol (i.e. without losses and noise, no thermal noise) with non-ideal state detection and finite two-mode squeezing. We write the ideal protocol in terms of block matrices. In the following, $I_2$ denotes the $2 \times 2$ identity matrix, $\hat{\sigma}_z$ denotes the Pauli $z$-matrix, $0_2$ is the $2 \times 2$ zero matrix and $\mathbf{0} = (0,0)^{\mathrm{T}}$. The covariance matrix $V$ and the displacement $d$ of the tripartite input state can then be expressed as

$$V = \frac{1}{4}\begin{pmatrix} I_2 \cosh 2r & \hat{\sigma}_z \sinh 2r & 0_2 \\ \hat{\sigma}_z \sinh 2r & I_2 \cosh 2r & 0_2 \\ 0_2 & 0_2 & I_2 \end{pmatrix}, \qquad d = \begin{pmatrix} \mathbf{0} \\ \mathbf{0} \\ d_{\mathrm{i}} \end{pmatrix}. \tag{S42}$$

The ideal 50:50 beam splitters, acting on Alice's side, are described by

$$B = \frac{1}{\sqrt{2}}\begin{pmatrix} \sqrt{2}\, I_2 & 0_2 & 0_2 \\ 0_2 & I_2 & I_2 \\ 0_2 & -I_2 & I_2 \end{pmatrix}. \tag{S43}$$

To model the phase-sensitive amplification of JPA 3 and JPA 4, we define the matrices

$$J_3 = \begin{pmatrix} 1/\sqrt{G} & 0 \\ 0 & \sqrt{G} \end{pmatrix} \qquad J_4 = \begin{pmatrix} \sqrt{G} & 0 \\ 0 & 1/\sqrt{G} \end{pmatrix} \tag{S44}$$

and

$$J = \begin{pmatrix} I_2 & 0_2 & 0_2 \\ 0_2 & J_3 & 0_2 \\ 0_2 & 0_2 & J_4 \end{pmatrix}. \tag{S45}$$

For the directional coupler, we write

$$C = \begin{pmatrix} \sqrt{1-\beta}\, I_2 & \sqrt{\beta}\, I_2 & 0_2 \\ -\sqrt{\beta}\, I_2 & \sqrt{1-\beta}\, I_2 & 0_2 \\ 0_2 & 0_2 & I_2 \end{pmatrix}. \tag{S46}$$

As a result, the ideal teleportation protocol can be expressed as

$$T = CBJB = \frac{1}{2}\begin{pmatrix} 2\sqrt{1-\beta}\, I_2 & \sqrt{\beta}(J_3 - J_4) & \sqrt{\beta}(J_3 + J_4) \\ -\sqrt{\beta}\, I_2 & \sqrt{1-\beta}(J_3 - J_4) & \sqrt{1-\beta}(J_3 + J_4) \\ 0_2 & -J_3 - J_4 & -J_3 + J_4 \end{pmatrix}. \tag{S47}$$

The final covariance matrix according to Eq. S47 is calculated by

$$V' = TVT^{\dagger}. \tag{S48}$$

After some lengthy calculations based on the aforementioned formalism, one can find the local covariance matrix $V_{\mathrm{f}}$ in path 1, corresponding to the output state of the directional coupler

$$V_{\mathrm{f}} = \frac{1}{16}\left\{4\cosh 2r I_2 + 2\sqrt{\beta}\sinh 2r(J_3 - J_4)\hat{\sigma}_z + 2\sqrt{\beta}\sinh 2r\hat{\sigma}_z(J_3 - J_4) + \beta\cosh 2r(J_3 - J_4)^2 + \beta(J_3 + J_4)^2\right\} \tag{S49}$$

If we now let

$$\beta \to 0, \qquad G \to \infty, \qquad G\beta = 4, \tag{S50}$$

we find that $J_3$ and $J_4$, combined with the coupling $\beta$, are transformed into the quadrature projection operators

$$\frac{\sqrt{\beta}}{2}J_3 \to \Pi_p = \begin{pmatrix} 0 & 0 \\ 0 & 1 \end{pmatrix}, \qquad \frac{\sqrt{\beta}}{2}J_4 \to \Pi_q = \begin{pmatrix} 1 & 0 \\ 0 & 0 \end{pmatrix}, \tag{S51}$$

where $\Pi_p$ ($\Pi_q$) describes a projective measurement of the $p$ ($q$) quadrature in the quadrature basis $(p, q)$. The beam splitter between the measurement JPAs and the directional coupler transforms the quadrature measurement basis $(p, q)$ to the hybridized measurement basis $(\tilde{p}, \tilde{q})$, where

$$\tilde{p}(p, q) = \frac{p + q}{2} \tag{S52}$$

denotes the symmetric hybridization and

$$\tilde{q}(p, q) = \frac{p - q}{2} \tag{S53}$$

denotes the antisymmetric hybridization. The terms symmetric and antisymmetric refer to the fact that $\tilde{p}(p, q) = \tilde{p}(q, p)$ and $\tilde{q}(p, q) = -\tilde{q}(q, p)$, i.e. $\tilde{q}(p, q)$ changes its sign when JPA 3 and JPA 4 are exchanged. Geometrically, this operation rotates the phase space by $\pi/4$. The qubit analogue of this operation would be a basis change from $z$ to $x$ via a $\pi/2$-pulse. The measurement operator $\Pi_+$ ($\Pi_-$) of the symmetric (antisymmetric) hybrid can be obtained with the beam splitter operation

$$\begin{pmatrix} \Pi_+ \\ \Pi_- \end{pmatrix} = \frac{1}{2}\begin{pmatrix} I_2 & I_2 \\ -I_2 & I_2 \end{pmatrix}\begin{pmatrix} \Pi_q \\ \Pi_p \end{pmatrix}, \tag{S54}$$

implying

$$\Pi_+ = \frac{\Pi_p + \Pi_q}{2}, \qquad \Pi_- = \frac{\Pi_p - \Pi_q}{2}. \tag{S55}$$

We note that $\Pi_+ = I_2/2$ and $\Pi_- = -\hat{\sigma}_z/2$, however, we keep the notation in terms of measurement operators to keep intuition. Under condition Eq. S50, we find for Eq. S49

$$V_{\mathrm{f}} = \frac{1}{4}\left\{\cosh 2r I_2 + 4\sinh 2r\Pi_-\hat{\sigma}_z + 4\cosh 2r\Pi_-^2 + 4\Pi_+^2\right\}. \tag{S56}$$

As a result, the local covariance matrix $V_{\mathrm{f}}$ of the final teleported state is given by

$$V_{\mathrm{f}} = \frac{1}{4}(2e^{-2r} + 1)I_2. \tag{S57}$$

Furthermore, the final displacement in path 1 coincides with the displacement of the input state, $d_{\mathrm{f}} = d_{\mathrm{i}}$. As a result, the teleportation fidelity $F$ can be expressed by the well-known result

$$F = \frac{1}{\sqrt{\det((e^{-2r} + 1)I_2)}} = \frac{1}{1 + e^{-2r}}, \tag{S58}$$

which reaches 1/2 in the classical case $r = 0$. In this case, we have $V_{\mathrm{f}} = 3I_2/4$, since we add the vacuum fluctuations from path 3 to path 1. In the following, we investigate the effect of finite squeezing and suboptimal measurement

gain. In this case, we reconsider the final covariance matrix and calculate the displacement without the assumption that the projection conditions Eq. S50 hold

$$V_\mathrm{f} = \frac{I_2}{16}\left\{ \cosh 2r \left[4(1-\beta) + \beta\left(\sqrt{G} - \frac{1}{\sqrt{G}}\right)^2\right] - 4\sqrt{\beta(1-\beta)}\left(\sqrt{G} - \frac{1}{\sqrt{G}}\right)\sinh 2r + \beta\left(\sqrt{G} + \frac{1}{\sqrt{G}}\right)^2\right\}. \tag{S59}$$

$$d_\mathrm{f} = \frac{\sqrt{\beta}}{2}\left(\sqrt{G} + \frac{1}{\sqrt{G}}\right)d_\mathrm{i}. \tag{S60}$$

We consider the classical case, hence

$$V_\mathrm{f} = \frac{I_2}{8}\left(2(1-\beta) + \beta G + \frac{\beta}{G}\right). \tag{S61}$$

From that, we obtain the result

$$F_\mathrm{c} = \frac{\exp\left(-|\alpha|^2 \frac{B(\beta,G)}{A(\beta,G)}\right)}{2A(\beta,G)}, \tag{S62}$$

with

$$A(\beta,G) = \frac{1}{8}\left(4 - 2\beta + \beta G + \frac{\beta}{G}\right), \tag{S63}$$

$$B(\beta,G) = \left(\frac{\sqrt{\beta}}{2}\left(\sqrt{G} + \frac{1}{\sqrt{G}}\right) - 1\right)^2. \tag{S64}$$

We first consider the case without displacement, $|\alpha|^2 = 0$. With $\beta \ll 1$, we obtain

$$F_\mathrm{c}(G,\beta) = \frac{4}{4 - 2\beta + \beta G + \beta/G}. \tag{S65}$$

We observe that $F(1,\beta) = 1$, as expected for vacuum teleportation. If we meet the projection condition $G\beta = 4$, we obtain the expected threshold $F = 1/2$ for $G \to \infty$, $\beta \to 0$. For finite $\beta$ and $G \to \infty$, we obtain $F \to 0$ since we strongly amplify Alice's part of the TMS (which locally looks like a thermal state) and hence cannot achieve destructive interference at the directional coupler. We assume that $\beta \ll 1$ and $G \gg 1$ and define the quantity $k = \beta G/4$. This quantity describes the "projectiveness" of the measurement. In the quantum case, $r \neq 0$, we then find the fidelity

$$F_\mathrm{q} = \frac{\exp\left(-|\alpha|^2 \frac{(\sqrt{k}-1)^2}{C(r,k)}\right)}{C(r,k)}, \tag{S66}$$

where we define the function

$$C(r,k) = (1+k)\cosh^2 r - \sqrt{k}\sinh 2r. \tag{S67}$$

The classical fidelity can be rewritten as

$$F_\mathrm{c} = \frac{\exp\left(-|\alpha|^2 \frac{(\sqrt{k}-1)^2}{1+k}\right)}{1+k}. \tag{S68}$$

---


* kirill.fedorov@wmi.badw.de
† Present affiliation: IQM, Nymphenburgerstr. 86, 80636 Munich, Germany
‡ frank.deppe@wmi.badw.de


[1] S. Pogorzalek, K. G. Fedorov, M. Xu, A. Parra-Rodriguez, M. Sanz, M. Fischer, E. Xie, K. Inomata, Y. Nakamura, E. Solano, A. Marx, F. Deppe, and R. Gross, Nat. Comm. **10**, 2604 (2019).
[2] K. G. Fedorov, S. Pogorzalek, U. Las Heras, M. Sanz, P. Yard, P. Eder, M. Fischer, J. Goetz, E. Xie, K. Inomata, Y. Nakamura, R. Di Candia, E. Solano, A. Marx, F. Deppe, and R. Gross, Sci. Rep. **8**, 6416 (2018).
[3] M. Renger, S. Pogorzalek, Q. Chen, Y. Nojiri, K. Inomata, Y. Nakamura, M. Partanen, A. Marx, R. Gross, F. Deppe, and K. G. Fedorov, (2020), arXiv:2011.00914 [quant-ph].
